# Supplementary material for: Mechanical, elastic and thermodynamic properties of crystalline lithium silicides
Source: arXiv:1610.08991 source file (2016-10-27)
Supplement: Supplementary file 1 [file supplementary_material.pdf]

# Supplementary material: Mechanical, elastic and thermodynamic properties of crystalline lithium silicides


Sebastian Schwalbe* and Jens Kortus
*Institute of Theoretical Physics, TU Bergakademie Freiberg, Leipziger Str. 23, D-09596 Freiberg, Germany*

Thomas Gruber
*Computational Quantum Chemistry for Solids, Max-Planck-Institut für Festkörperforschung, University of Stuttgart, Heisenbergstraße 1, D-70569 Stuttgart, Germany*

Kai Trepte
*Theoretical Chemistry, Technische Universität Dresden, Bergstraße 66b, D-01062 Dresden, Germany*

Franziska Biedermann and Florian Mertens
*Institute of Physical Chemistry, TU Bergakademie Freiberg, Leipziger Str. 29, D-09599 Freiberg, Germany*



(Dated: October 27, 2016)



* schwalbe@physik.tu-freiberg.de

### A1 Calculation parameters

TABLE A1: DFT parameters

| $Li_xSi_y$ | cutoff [Ry] | k-grid |
|---|---|---|
| Si | 50 | 12x12x12 |
| $Li_{12}Si_7$ | 70 | 5x2x3 |
| $Li_7Si_3$ | 80 | 16x16x4 |
| $Li_{13}Si_4$ | 70 | 8x4x16 |
| $Li_{15}Si_4$ | 70 | 6x6x6 |
| $Li_{21}Si_5$ | 70 | 4x4x4 |
| $Li_{17}Si_4$ | 70 | 4x4x4 |
| $Li_{22}Si_5$ | 70 | 4x4x4 |
| Li | 50 | 24x24x24 |

TABLE A2: LAMMPS parameters

| $Li_xSi_y$ | supercell size |
|---|---|
| Si | 3x3x3 |
| $Li_{12}Si_7$ | 2x2x2 |
| $Li_7Si_3$ | 3x3x6 |
| $Li_{13}Si_4$ | 3x3x3 |
| $Li_{22}Si_5$ | 3x3x3 |
| Li | 12x12x12 |

### A2 Radial pair distribution function

To validate that the right crystal structures are used for our MD investigations, the radial pair distribution function (RPDF) was calculated for the initial MD structure, the averaged MD structures, the final MD structure and compared with the corresponding experimental structure for all investigated phases (see FIG. A1). We observe that the initial MD structure perfectly match the experimental structure. Furthermore we can conclude that our MD runs are long enough, because the final MD structure is in good agreement with the averaged MD structure for all investigated structures.

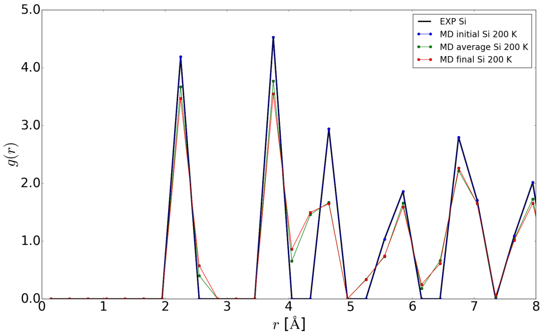


(a) Si $g(r)$ 200K

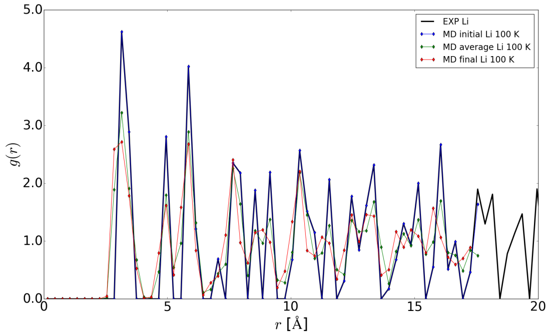


(b) Li $g(r)$ 100K

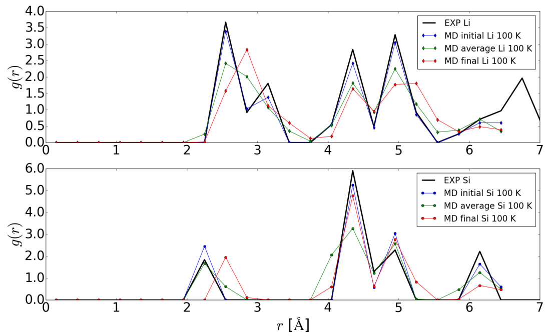


(c) $Li_7Si_3$ $g(r)$ at 100K

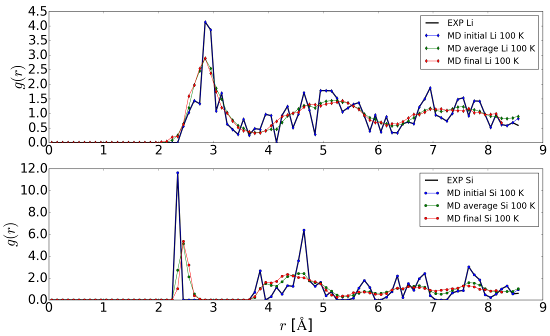


(d) $Li_{12}Si_7$ $g(r)$ at 100K

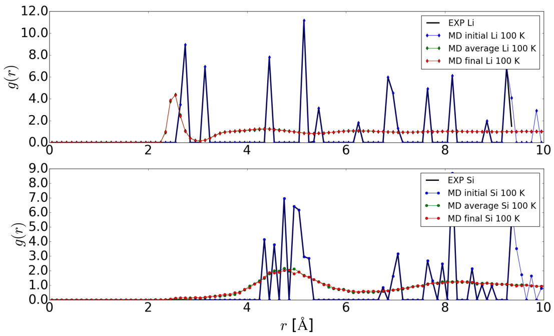


(e) $Li_{22}Si_5$ $g(r)$ at 100K

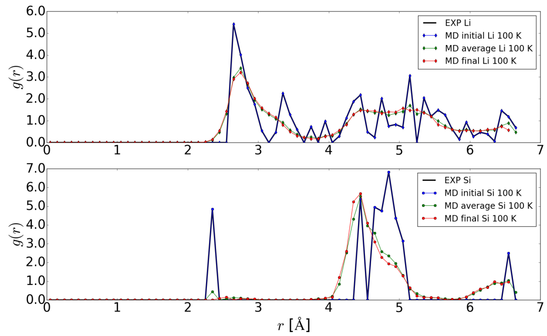


(f) $Li_{13}Si_4$ $g(r)$ at 100K

FIG. A1: The radial pair distribution function (RPDF) is evaluated for the initial structure, the average over all structures produced for one MD run and for the last structure of the MD run for pure elements (silicon in (a) and for lithium in (b)) and the lithium silicides ($Li_7Si_3$ in (c),$Li_{12}Si_7$ in (d), $Li_{22}Si_5$ in (e) and $Li_{13}Si_4$ in (f)). For each system (see TAB. A A2) a corresponding supercell is created for the experimental structure to have comparable neighbour spheres.
